# Supplementary material for: LATMiX: Learnable Affine Transformations for Microscaling Quantization of LLMs
Source: arXiv:2602.17681 source file (2026-04-23)
Supplement: Supplementary file 1 [file analysis_toy_example.tex]

\begin{figure*}
% \centering
% \renewcommand{\arraystretch}{1.0}
% \setlength{\tabcolsep}{6pt}
% ---- Column labels (A-D) ----
% \begin{tabular}{c c c c c}
%  & \textbf{A} & \textbf{B} & \textbf{C} & \textbf{D} \\
% \end{tabular}

% \vspace{4pt}
% ---- 3x4 grid with row labels (Case I-III) ----
\begin{tabular}{ c c c}
  \textbf{Vanilla} & \textbf{B} & \textbf{Block}  \\
{\includesvg[width=0.30\linewidth]{images/example_learn/case_0_vanilla_block_example.svg}} &
{\includesvg[width=0.30\linewidth]{images/example_learn/case_0_h_block_example.svg}} &
{\includesvg[width=0.30\linewidth]{images/example_learn/case_0_hb_block_example.svg}}  \\[6pt]

{\includesvg[width=0.30\linewidth]{images/example_learn/case_1_vanilla_block_example.svg}} &
{\includesvg[width=0.30\linewidth]{images/example_learn/case_1_h_block_example.svg}} &
{\includesvg[width=0.30\linewidth]{images/example_learn/case_1_hb_block_example.svg}} 
\end{tabular}

\caption{A 3$\times$4 panel figure with row labels (cases) and column labels (A--D).}
\label{fig:cases_3x4}
\end{figure*}
