# Supplementary material for: LATMiX: Learnable Affine Transformations for Microscaling Quantization of LLMs
Source: arXiv:2602.17681 source file (2026-04-23)
Supplement: Supplementary file 2 [file vllm.tex]

\section{Performance Evaluation Using vLLM Hardware Simulation}
\label{apx:vllm}

\todo[inline]{Feel in text and add reference from main where is relevant}

\begin{figure}[!h]
    \centering
     \includesvg[width=0.9\linewidth]{images/qwen32_comp_throughput.svg}
    \caption{Throughput of different approaches.}
    \label{fig:throughput}
\end{figure}
